# Supplementary material for: Improving High Contention OLTP Performance via Transaction Scheduling
Source: arXiv:1810.01997 source file (2018-10-03)
Supplement: Supplementary file 1 [file correlation-clustering.tex]

\section{Correlation Clustering}
\applabel{correlation-clustering}
